# Supplementary material for: Privacy Engineering Meets Software Engineering. On the Challenges of Engineering Privacy ByDesign
Source: arXiv:2007.08613 source file (2020-07-16)
Supplement: Supplementary file 1 [file EPbDMethodologies.tex]

\subsection{PbD as practice: Privacy papers and the SDL / (micro)services}

\subsubsection{Risk assessment/Threat modeling}

The LINDDUN methodology is an approach for modeling privacy threats \cite{DengWSPJ11}. The methodology includes the anti-property or threat for two types of privacy properties: soft (content unawareness, policy and consent noncompliance) and hard (likability, identifiability, non-repudiation, detectability, and disclosure of information). LINDDUN is influenced by STRIDE \cite{Shostack14}, a security modeling method with trees of threats and data flow diagrams created for each category of threats. It is possible to use the LINDDUN as a reference guide for privacy threats but lacks the mapping to a software development process and a comprehensive view of the organizational goals linked with the privacy goals.

\subsubsection{Goal-oriented}

In their work, Liu and colleagues present privacy and security from the point of view of requirements engineering \cite{LiuYM03}. Privacy is a non-functional requirement that affects the design of the system, which is modeled with i*, a goal-oriented modeling method. Their approach is to transform OECD's categories into goals and to then, create a reference catalogue with privacy solutions addressing each privacy goal. The catalogue is high-level motivational analysis (consisting of actors who have goals and soft goals, and who take actions to achieve their goals). The actions for satisfying the different goals are not universal and are arbitrarily chosen to show a proof-of-concept for modeling privacy requirements. The works merits include contextual analysis capabilities and structural consistency based on a requirements engineering modeling method. With the modeling method, it is possible to present dependencies between goals (of the same actor or of different actors), to model the viewpoints of different actors and other non-functional requirements.

PriS proposes a holistic approach that connects `high-level' organizational goals and `privacy-compliant' IT systems \cite{KalloniatisKG2008}. PriS first models privacy requirements from an organizational point of view in the form of organizational goals (GORE) and then, using seven predefined privacy-process patterns describes the impact of the privacy goals on the organizational processes and the IT systems. The Formal PriS method also defines four activities to carry out the design: (1) elicit privacy-related goals, (2) analyse the impact of privacy goals on organizational processes, (3) model affected processes using privacy-process patterns, (4) identify the techniques that best support/implement privacy-related processes. The authors identify the gap between design and implementation and the lack of support given to developers to implement privacy requirements into their systems. PriS is a methodology rather than a recipe book -- it uses models and principles of refinement and abstraction between levels to connect different areas/domain involved in system design. However, PriS lacks the mechanism to integrate this design process into an iterative software development. PriS does not consider the type of software system to be developed: there is no discrimination between a monolith and a service-oriented system, hence, there are no guidelines how to reason about modular ever-changing system. Also, even though, the authors list several PETs ``implementing'' the eight privacy requirements, the list is limited to technologies and not to classes of technologies, which makes it unsuitable for extending. The leap between the privacy process patterns and the PETs is non-trivial and even though the authors set for themselves the goal to provide a methodology that does not give a static recipe but a heuristics-based holistic approach to integrate privacy into IT systems, it is unclear how to break out of the pre-defined privacy requirements, the pre-defined privacy-process patterns, or the pre-defined PETs mapping. Privacy is loosely defined: it is a specialized organizational goal or a requirement. However, there are eight privacy goals that are assumed to be a given even though the first activity in the methodology is to identify privacy goals (authorization, authentication, identification, anonymity, data protection, pseudonymity, unlinkability, and unobservability).

Hansen et al. introduced the notion of protection goals to create ``a feature-complete model for evaluating an IT system's impact on all aspects of privacy and data protection'' \cite{HansenJR15}. The privacy goals are six and include three well-established goals from security (confidentiality, integrity, availability, or CIA) and the newly relevant goals of privacy and data protection (unlikability, transparency, and intervenability). The authors discriminate between privacy and data protection; privacy take on the perspective of an individual, whereas data protection is an organization-centered view.  The goals are complimentary w.r.t. achieving privacy in an ideal world but as the authors point out, these goals are contradictory and depending on the technology that implements them, might be exclusive. For example, transparency and linkability are of conflicting nature, as the former requires monitoring of the actual processing by, for example, logging various actions, but the latter promotes avoidance of such information being recorded to minimize the risk of misuse. The work mentions the challenges of using external services by providing data in the clear only to introduce some techniques (e.g. secure computation and homomorphic encryption). The challenges for software developers to reason about privacy and data protection are not mentioned.

\subsection{Software Development/System Design}

Hoepman defines privacy design strategies to help IT engineers solve recurring software development problems in the light of 'privacy-by-design' development \cite{Hoepman14}. The first observation we make is that the author assumes that privacy and data protection are synonyms. From then on, to aid the IT architects, Hoepman derives privacy design from legislation (e.g., OECD guidelines, the 1995 European data protection directive) and maps them to (privacy) design patterns that help implement the strategy. There are eight privacy design strategies related either to the data (minimize, separate, aggregate, hide) or to the process (inform, control, demonstrate, enforce). Our next observation is that the privacy design patterns are not complete; there are some suggestions (select before collect, mix networks, etc.) but the author gives no comprehensive list later to be categorized as a pattern for one or another strategy. Moreover, the privacy design patterns are not software design patterns. For example, encryption (a privacy pattern for the hide strategy) is a technique rather than ``a schema for refining the subsystems or the components of a software system, or the relationship between them'', which is the definition of a design pattern the author adopted in their paper. For a non-expert privacy engineer, this terminology would be misleading. Other privacy strategies lack design patterns altogether, e.g. separate. Moreover, the strategies do not describe how to engineer privacy by design in an agile software development process or how to compose applications from various components. There is no mention of how to evolve a software iteratively, which is the pre-dominant industry case.

Spiekermann and Cranor discuss the practical implications of engineering privacy and what the shift from privacy from the physical to the digital world might entail \cite{SpiekermannC09}. In their work, the authors propose the use of a privacy sphere - a privacy space for users, recipients, and a joint sphere. The spheres help us reason about the privacy constraints and concerns within the boundaries of each sphere. Moreover, Spiekermann and Cranor devise a system design method for including privacy in the design. At the first two stages of the system design, the authors propose that privacy be addressed with the help of policies. At the last two stages - with the help of architectural choices. The policies are a light-weight privacy mechanism as they ensure not so much privacy as compliance. As for the architectural choices, they are explained in detail but are disconnected from the practical work of a developer, i.e. who would find them as a prescription only to a subset of architectural choices they need to make, hence, rendering the architectural choices unactionable. A curious caveat in this work is the term privacy-friendly systems, that the authors coined to name systems that include privacy in their design but not necessarily in the traditional privacy-preserving or enhancing meaning that is mostly in use today.

Al-Momani et al. present a software development process (V-model) augmented for engineering privacy \cite{Al-MomaniKSKB19}. The privacy-aware V-model, called W-model, starts with privacy impact assessment in order to elicit privacy threats and to find countermeasures to remedy these threats. The W-model introduces two privacy-centric stages: privacy analysis and privacy-enhanced architecture. All the other stages of the classic V-model are ``privacy-enhanced.'' The privacy analysis during the W-process is when the privacy engineers elicit the privacy threats and select countermeasures for them. The countermeasures should be integrable in the system and compatible with other countermeasures, which are requirements not often mentioned regarding PETs when methodologies on PbD explain how to select the right one for the job. The next step, privacy-enhanced architecture, is dedicated to design a high-level and a low-level system architecture that meets the business and privacy requirements. However, the design phase and the implementation phase are disconnected and even though there is short mention on how privacy and systems engineers resolve issues arising during the implementation phase, the recommendation is that the interaction between system and privacy engineers should be on critical aspects in order to increase the time-efficiency. The claim of the authors is that the enhanced privacy culture of the companies via the component "environment and infrastructure" will reduce unnecessary communication. The paper mentions nothing regarding services and modules that interact with the PETs, only that the PETs need to be integrable in a system.

PEARs attempts to answer the question how to engineer PbD on the architectural level of an application \cite{Kung14}. As most software architecture text, it's abstract and completely out of the blue, no idea where the architectural tactics and patterns come from. Kung proposes to use a separation between NFR (how the system does it) and FR (what the system does) which is arbitrary (because such a separation does not exist). For example, FRs includes purpose limitation. Why? Why this is not an NFR? NFRs include minimization. Why? Then, the architecture is supposed to be related to some tactics that are associated with technologies and patterns. There are 4 tactics mentioned in the paper - minimization, enforcement, accountability, modifiability (unjustified where they come from). My guess is that the NFR are the source for the tactics, but this is not written explicitly. It's written that the architecture depends of NFRs but the 4 tactics are just examples and not an exhaustive taxonomy of other NFRs that can be translated into tactics for the architecture, even though the Kung describes these tactics as a proposal. The selection of the right tactics is said to be "art of selecting " and to depend of the available PETs and the cost effectiveness. No further intuition is given how to select. The paper includes 3 examples of patterns (user data confinement, hippocratic management, isolation) that are unrelated to the 4 tactics. Architecture is supposed to be evaluated with a PIA; there are 5 sentences in total that describe how this evaluation will be done. The PbD process that integrates architectural design is a linear except for one loop that connects the architecture and the privacy FRs. There is no development in the PbD process, neither the process is considered to be of any iterative nature. The process ends with the evaluation of privacy (PIA). There is no mention of composition of the software (services), how to integrate changes, context of use, development activities.
