# Supplementary material for: Privacy Engineering Meets Software Engineering. On the Challenges of Engineering Privacy ByDesign
Source: arXiv:2007.08613 source file (2020-07-16)
Supplement: Supplementary file 2 [file EPbDTable.tex]

\begin{table*}[t]
    \begin{tabular}{|c|c|c|c|c|c|c|c|c|c|c|c|c|}
        \hline
        
        \textbf{} & \rotatebox{90}{\textbf{Services}} & \rotatebox{90}{\textbf{Waterfall}} &  \rotatebox{90}{\textbf{Integration}} & \rotatebox{90}{\textbf{Changes}}  & \rotatebox{90}{\textbf{Heuristics}} & \rotatebox{90}{\textbf{Prescribe}}  & \rotatebox{90}{\textbf{\makecell{Minimize\\data}}} & \rotatebox{90}{\textbf{\makecell{Mapping\\to PETs}}}  & \rotatebox{90}{\textbf{\makecell{Risks/\\threats} }}& \rotatebox{90}{\textbf{\makecell{Goal-\\oriented} }} & \rotatebox{90}{\textbf{\makecell{Context \\of use}} } & \rotatebox{90}{\textbf{\makecell{Intended \\audience}} }\\ \hline
        
        \multicolumn{13}{|c|}{\textbf{Academic publications}}  \\ \hline 
        
        Hoepman (Privacy strategies) \cite{Hoepman14} & \Circle & \RIGHTcircle & \Circle & \Circle & \CIRCLE & \RIGHTcircle  & \RIGHTcircle & \CIRCLE  & \Circle  & \Circle & \Circle & Eng \\ \hline
        
        Deng et al. (LINDDUN) \cite{DengWSPJ11} & \Circle &  \CIRCLE & \Circle  &  \Circle &  \Circle &  \CIRCLE & \Circle & \CIRCLE & \CIRCLE &  \Circle & \Circle & Org/Academic \\ \hline
        
        Spiekermann and Cranor \cite{SpiekermannC09} & \CIRCLE & \CIRCLE &  \Circle &  \Circle &  \Circle &  \CIRCLE & \Circle & \Circle & \Circle & \Circle & \RIGHTcircle & Eng/Academic\\ \hline
                
        PRIAM \cite{DeM16} & \CIRCLE & \CIRCLE &  \Circle &  \Circle &  \Circle &  \CIRCLE & \RIGHTcircle & \Circle & \CIRCLE & \Circle & \CIRCLE & Org \\ \hline
                
        Hansen et al. (Protection goals) \cite{HansenJR15}  &  \CIRCLE & \CIRCLE &  \Circle &  \Circle &  \Circle &  \CIRCLE & \RIGHTcircle & \Circle & \Circle & \RIGHTcircle & \Circle & Org/Academic\\ \hline
        
        G\"urses et al. (EPbD) \cite{GursesTD11,GursesTD15} &  \Circle &  \CIRCLE &  \Circle & \Circle &  \CIRCLE  & \Circle  &  \CIRCLE  &\CIRCLE & \CIRCLE  &  \Circle &  \Circle & Org/Eng\\ \hline
        
        Al-Momani (W process) \cite{Al-MomaniKSKB19} & \Circle & \CIRCLE &  \Circle &  \RIGHTcircle &  \RIGHTcircle &  \Circle & \RIGHTcircle & \Circle &  \Circle & \CIRCLE & \Circle & Eng/Org/Academic \\ \hline
        
        Bernsmed (Applying EPbD)\cite{Bernsmed16}  & \CIRCLE & \CIRCLE & \Circle  &  \CIRCLE  &  \Circle &  \CIRCLE & \Circle & \Circle & \Circle & \Circle & \CIRCLE & Org \\ \hline
        
        Liu et al. (i*) \cite{LiuYM03} & \Circle & \CIRCLE &  \Circle &  \Circle &  \Circle &  \Circle & \Circle & \Circle &  \Circle & \CIRCLE & \CIRCLE & Org/Academic \\ \hline
        
        Kalloniatis (PriS method) \cite{KalloniatisKG2008} &  \Circle & \CIRCLE &  \Circle &  \RIGHTcircle &  \RIGHTcircle &  \Circle & \RIGHTcircle & \Circle &  \Circle & \CIRCLE & \Circle & Eng/Org/Academic \\ \hline

        Kroener and Wright \cite{KroenerW14} & \multicolumn{12}{|c|}{SoK\footnote{SoK - Summarization of Knowledge. We use the term in the broad sense to mean that the work provides an overview of the field.}  focused on the area of privacy by design in general} \\ \hline 
        
        Wueyts et al. \cite{WuytsSLJ19} & \multicolumn{12}{|c|}{SoK focused on threat elicitation} \\ \hline \hline

        \multicolumn{13}{|c|}{\textbf{Standards}}  \\ \hline 
        
        ISO 27550 \cite{ISO27550}  & \CIRCLE & \CIRCLE & \CIRCLE  &  \CIRCLE  &  \RIGHTcircle &  \Circle & \CIRCLE & \RIGHTcircle & \RIGHTcircle & \CIRCLE & \RIGHTcircle & Org/Eng \\ \hline
        
        OASIS PMRM \cite{PMRM13} & \CIRCLE  & \RIGHTcircle & \RIGHTcircle  &  \CIRCLE  &  \Circle &  \CIRCLE & \CIRCLE & \Circle & \RIGHTcircle & \Circle & \CIRCLE & Org/Eng \\ \hline
        
        Risk assessment in federal systems \cite{NISTIR8062} & \Circle & \Circle & \Circle  &  \Circle  &  \Circle &  \RIGHTcircle & \Circle & \Circle & \CIRCLE & \Circle & \CIRCLE & Legal \\ \hline
        
        OASIS Cavoukian \cite{CavoukianCJSDFFF14}  & \CIRCLE & \RIGHTcircle & \Circle  &  \Circle  &  \Circle &  \CIRCLE & \Circle & \Circle & \CIRCLE & \Circle & \CIRCLE & Org \\ \hline
        
        PRIPARE \cite{NotarioCMAMAKKW15}  & \Circle & \Circle & \Circle  &  \Circle  &  \Circle &  \CIRCLE & \Circle & \Circle & \CIRCLE & \CIRCLE & \CIRCLE & Org \\ \hline
        
        NISTIR 8062 \cite{NISTIR8062}  & \Circle & \Circle & \Circle  &  \Circle  &  \Circle &  \RIGHTcircle & \Circle & \Circle & \CIRCLE & \Circle & \CIRCLE & Org/Legal \\ \hline
    
    \end{tabular}
    
    \caption{Analysis of different engineering privacy by design methodologies according to twelve criteria. We used the following encoding: \Circle - the work does not consider or present this dimension, \RIGHTcircle - the work mentions this dimension but does not center around it, \CIRCLE - the work revolves around and analyzes in detail this dimension.}
    \label{table: epbd-methodologies-all}
    
\end{table*}
