# Supplementary material for: Privacy Engineering Meets Software Engineering. On the Challenges of Engineering Privacy ByDesign
Source: arXiv:2007.08613 source file (2020-07-16)
Supplement: Supplementary file 3 [file Services.tex]

% !TeX root = ../Agile_PbD.tex
A service is an overloaded term in the literature. 
We present here the definitions from the service science and the service-oriented computing communities. 

The service-oriented computing paradigm defines services as ``self-describing, platform-agnostic computational elements that support rapid, low-cost composition of distributed applications'' \cite{Papazoglou03}.
Service-oriented computing has been extended recently to microservices.
A microservice is still a service but highly specialized and independent \cite{DragoniGLMMMS17}
The definition of microservices vary but stay within the bounds of ``independent deployment and isolated development'' \cite{microservices}.
The most recent research in the area  push the boundaries on how small a (micro)service can be. 
These inquiries include the concept of serverless computing, sometimes called a function-as-a-service, \cite{BaldiniCCCFIMMRSS17} and questions on how small a computation outsourced to a cloud can be if it still needs to make sense \cite{LeeO19}.

Microservices architecture is a software architecture in which components are lightweight microservices that communicate through heterogeneous protocols \cite{DragoniGLMMMS17}.
The composition of microservices requires coordination done via an orchestration or a choreography composition pattern \cite{DragoniGLMMMS17}. 
In the case of orchestration, there is an engine that orchestrates the microservices and leaves less logic in the individual computing units who to contact next.
In the case of choreography, the individual microservices have the embedded logic that they use to invoke other microservices \cite{CernyDT17}. 
According to Alshuqayran et al. some of the pros of the microservices architecture are increase in agility, developer productivity, resilience, scalability, reliability, maintainability, separation of concerns, and ease of deployment \cite{AlshuqayranAE16}. 
There are, however, challenges to the microservices architecture, i.e., service discovery, security management, communication optimization, data sharing, and performance .

Moreover, the \textit{context} of the system, i.e. how the microservices are used in a full system, disappears when a monolith is broken into the smallest pieces that still hold together \cite{CernyDT17}.
Each individual microservices maintain only its own context, meaning, it has a consistent state within itself.
This microservices context, or bounded context, a notion from domain-driven design \cite{Evans04}, corresponds to the minimal amount of information that the service needs to `know' in order to be able to deliver its functionality.
This lack of visibility over the context of the system and a consistent state, can make it impossible to reason about the system as a whole or to design a system with some desired high-level properties. 

Microservices arose from industry as a way for teams to deliver their software independent of other teams \cite{Zimmermann17}. 
We can trace this to Conway's law that states that an IT system starts reflecting the structure of the organization that designs the system \cite{Conway68}.
Following this argument, it is not surprising that the small functional teams that govern their development with agile methodologies and that steer clear from any complex upfront design end up using the microservices paradigm to package their deliverables.
Microservices architecture is primarily used to enable independent service deployments and evolution.
The duality of the organizational context and the information systems integrated in this context is a known challenge \cite{Nuseibeh01}.

Even though some express the opinion that the service-oriented computing and the microservices paradigm are too close to be discerned as separate disciplines (cf. \cite{Zimmermann17}), the two still represent different concepts.
Inline with this, we define a \emph{microservice} to be the smallest IT service that is invoked in different components of an application, and a \emph{service} to be a means to deliver value to a service adopter.
A service, as defined by ITIL is ``a means of delivering value to customers by facilitating outcomes customers want to achieve without the ownership of specific costs and risks'' \cite{ITIL2011}. biz and technical at the same time and business agility\footnote{ITIL 2019 introduces a new definition which we will not use.}.
Based on this definition, the service value is closely related to the displacement of costs and risks from the customer to the service provider.
