# Supplementary material for: Privacy Engineering Meets Software Engineering. On the Challenges of Engineering Privacy ByDesign
Source: arXiv:2007.08613 source file (2020-07-16)
Supplement: Supplementary file 4 [file Standards.tex]

\subsection{Standards}
There are three main sources of standards for privacy and privacy by design: (1) International Standardization Organization (ISO), (2) Organization for the Advancement of Structured Information Standards (OASIS), and (3) National Institute of Standards and Technologies (NIST). In this section, we discuss the advancements that the standardization bodies have made and argue that in the most part existing standards and on-going standardization efforts neither resolve nor even touch upon the topics of the disconnect between software engineering, as in service-oriented and agile development trends, and privacy engineering practices. One additional observation is that standards are not representative of the entire privacy community as the researchers who specialize in privacy engineering are usually not a part of the standardization process. We also conclude that standards are coming as an upfront prescription of how privacy engineering should be done before there is a consensus within the research and industry communities on what privacy engineering is and how it should be conducted.

The ISO/IEC 29101:2018 \cite{ISO29101} standard defines a privacy architecture framework that specifies concerns regarding PII processed by an ICT systems, lists and connects components for the implementation of such systems. The framework is intended to be a technical reference for developers of ICT systems that process PII. The architecture consists of actors, components, and concerns, as well as interactions between components. The component view (technical architecture) is presented in three layers: privacy settings, identity management and access management, and PII. The views and layers are connected to the privacy principles of ISO/IEC 29100:2011 \cite{ISO29100}. The architecture is a concise representation of a lot of enterprise process interactions w.r.t. defining how to handle data. The roles of the stakeholders (principal,  controller, handler) as well the views that defines actors, systems, and interactions between these, are a stepping stone for an architecture of a privacy solution. However, the language of the standard remains legal and organizational, even though it is intended for developers to organize and develop systems that handle PII. The mapping to PETs is recommended but not specified in enough details, the PII layer mentions some technologies but has no reference list. The relationship between the layers of the components is represented visually with block/layered diagrams, and the only other relationship is the transitive one between the privacy principles and the layers. However, these two are insufficient to draw a conclusion which PET to use when and how to design the ICT system in the first place. There is no mention of the type of system (monolith or service-oriented) or the software development cycle. The standard relies heavily on the previous iteration of the 29100:2011 to define the requirements, the privacy process, etc. Also, the responsibilities to the developers are highly unrealistic - obtaining consent from PII principals is not only an engineering decision, neither is eliciting requirements, nor is communicating the purpose of PII collection, all of which are defined as concerns that developers should take care of.

Currently under development, the ISO/IEC TR 27550 \cite{ISO27550} is a draft for a standard on privacy engineering for system life cycle processes. The integration of privacy into the engineering of systems starts with introducing privacy concerns into the life cycle processes. The core is the integration of privacy into the concepts from ISO/IEC/IEEE 15288:2015 on system life cycle processes. The processes include: acquisition, supply, human resource management, knowledge management, risk management, stakeholder needs and requirements, system requirements definition, architecture, design. The processes excludes any system and software development activities after the design of the system; so what is left out of the life cycle is any development, testing, integration, maintenance, etc. This division of design and architecture and system building is a characteristic of a waterfall-style development and much less likely to occur in current software development practices. In an annex to the main document, there is a proposition how to integrate privacy into agile software development practices and the difference between a waterfall and agile development (agile is seen as iterative waterfall): privacy concerns are added to the system under development (which is to say that the backlog includes development plans for privacy). No explanation is given on what those development plans for privacy are. There is also a dedicated role in the Sprint process called product privacy owner, who might be an external or internal member of the team and who is responsible for privacy within the organization (not within the project).

NISTIR 8062 is a document that introduces the concepts of privacy engineering and risk management for federal systems \cite{NISTIR8062}.The goals are to establish a common vocabulary through which to promote understanding and communication of privacy risk and effective implementation of privacy principles. The document is mostly a road map that provides definitions (privacy engineering, privacy as an attribute of trustworthy systems, privacy objectives), an argument how privacy engineering could benefit from systems engineering, and some should-have's for the future (e.g., ``System designers and engineers, working with policy teams, can use the objectives to help bridge the gap between high-level privacy principles and their implementation within systems.'') The privacy objectives (predictability, manageability, disassociability) are a hypothetical step towards making privacy principles actionable, as the objectives are defined as measurable outcomes to provide system engineers with clarity what privacy engineering dictates what behavior the system should exhibit. The objectives are mapped to FIPPs (Fair Information Practice Principles) to show the decomposition of high-level principles to system properties. Yet, these objectives are highly dependent on the context of the system and no guidance is provided for system engineers on how to conduct the analysis (besides a risk analysis) that would potentially yield requirements that satisfy these objectives. The choice of these three objectives as opposed to any other property and any other number of objectives, is not justified. The document provides a privacy risk model that defines some additional vocabulary, e.g., problematic data action, privacy risk factors, privacy risk characteristics, and most interestingly (for the sake of our paper) context: ``Context—the circumstances surrounding the system's processing of PII—is the foundation for the interpretative analysis necessary to understanding when a privacy boundary line has been crossed.'' This means there is an understanding of the fluidity of the context of use of ICT systems, and for that, the privacy engineering measures would be specific for each case, however, NISTIR 8062 says little about how system engineers should independently of privacy experts think about privacy, analyze, design, develop and evaluate their systems w.r.t. the changing context of use.

The PRIPARE methodology is a reference guide whose purpose it is to integrate existing privacy engineering practices and contribute a consistent body of knowledge that is easy-to-use by software engineers \cite{NotarioCMAMAKKW15}. The methodology is built on top of the traditional waterfall software development process but uses an iterative version for the phases. The different software development phases are linked with comprehensive activities and best practices for privacy engineering. The handbook connects the relevant laws and the engineering activities more closely than other methodologies. One of the missing points is the iterative development process (even though it is mentioned that the software architecture would be designed iteratively, no details are given); the methodology claims to be applicable in the case of change in the requirements for the system.
