# Supplementary material for: Privacy Engineering Meets Software Engineering. On the Challenges of Engineering Privacy ByDesign
Source: arXiv:2007.08613 source file (2020-07-16)
Supplement: Supplementary file 5 [file AgileMethodsHistory.tex]

\subsection{Agile development: A New World}
Since the beginning of software engineering in the late 60s, a variety of management and engineering literature proposed wildly different models on how to produce software. Until the 1990s, structured processes, such as the waterfall or spiral model, dominated the industry. These models rely on rigorously regimented practices, extensive documentation, and detailed planning and management \cite{EstlerNFMS14}. In \emph{waterfall models}, as the US Department of Defense standardized the term, software projects have a clear beginning during which the requirements and design are settled, and a final stage during which a version of a software is tested and released to its users. 

Starting with the 1980s, and continuing with the 1990s, programmers started proposing more \emph{lightweight} models that promoted greater autonomy for developer teams, questioning the predominantly managerial approaches to software development. Scrum, Rational Unified Process, Extreme Programming presented turning points in these developments. Some of these methodologies focus on techniques (e.g., pair-programming), while others focus on managerial processes (e.g., stakeholder involvement, stand-up meetings), with an overall emphasis on continuous testing (starting with test codes and extending to integration testing), communication and visibility of progress (Parson 2011). 

We use \emph{agile methodologies} as an umbrella term to refer to this latter variety of approaches to software development that contrast with what are called Big Design Up Front models, and that emphasize iterative customer centered engineering of functionality. We shorthand these methods as agile inspired by one of these proposals which culminated in what was titled the ``Manifesto for Agile Software Development'' in 2001 \cite{beckBCCFGHHJKMMMSST2001}. The supporters of this manifesto value:
\begin{quote}
Individuals and interactions over processes and tools\\
                               Working software over comprehensive documentation\\
      Customer collaboration over contract negotiation\\
    	        Responding to change over following a plan \cite{beckBCCFGHHJKMMMSST2001}.\\

\end{quote}

Like many of its contemporaries, the manifesto underlines a ``no design up front'' attitude. Instead, it proposes to produce software in much shorter iterations (weeks vs years, or multiple times a day), in greater simplicity (always do the simplest thing that could possibly work and don't design more than what you need right now), and continuous code reviews \cite{FoxP13}. This leads to increased emphasis on modularity, incremental design, iterations in feature development that are open to changing requirements, and continuous deployment, i.e., releasing code as frequently as possible. Another important effect is the removal of documentation efforts, assuming that development must modularize and simplify code, ideally, to the extent of making documentation redundant. 

Agile methods are as much about development efficiency as they are about the success of software based businesses. In addition to enabling customer centricity, agile methods promise to give companies control over the costs of maintenance, monitoring, and support. Instead of waiting for the release of new versions, users can benefit from continuous updates. This produces a big advantage in an industry where as much as 60 percent of software costs are for maintenance, and of those costs 60 percent are for adding new functionality to legacy software (Armando and Patterson 2013).

Some methods make the connection between business interests and development methodologies even more evident. Especially development methods inspired by processes used in traditional manufacturing, e.g., Kanban, lean manufacturing were key to aligning business models, key performance indicators (KPIs) with rapid feature development driven by feedback from users or customers. As a result, data that could be used to measure user interactions and interest became a necessary part of optimizing features, fulfilling KPIs and pivoting companies effectively towards more promising business models.

Finally, despite their anti-managerial gist, proposals for agile methodologies were aligned with then new management theories which erred on the side of ``multidisciplinary teams''  that work more like a rugby team engaged in iterative experimentation across all phases of production simultaneously as a way to achieve speed and flexibility in production. In addition to enabling programming and business on demand, these methods were invaluable in addressing the inflexibility of planned development that proved to lead to grand failures and brittleness in managing uncertainty. Agile methodologies also promoted a much more experimental approach to software engineering, relying on user data and feedback for enabling these experiments.
